# Supplementary material for: SIMMC 2.0: A Task-oriented Dialog Dataset for Immersive Multimodal Conversations
Source: arXiv:2104.08667 source file (2021-10-20)
Supplement: Supplementary file 1 [file main_suppl.tex]

%
% File emnlp2020.tex
%
\documentclass[11pt,a4paper]{article}
\usepackage[hyperref]{emnlp2020}
\usepackage{times}
\usepackage{latexsym}
\renewcommand{\UrlFont}{\ttfamily\small}
\usepackage[dash,dot]{dashundergaps}
\usepackage{url}


% This is not strictly necessary, and may be commented out,
% but it will improve the layout of the manuscript,
% and will typically save some space.
\usepackage{microtype}

%\aclfinalcopy % Uncomment this line for the final submission
\def\aclpaperid{2996} %  Enter the acl Paper ID here

%\setlength\titlebox{5cm}
% You can expand the titlebox if you need extra space
% to show all the authors. Please do not make the titlebox
% smaller than 5cm (the original size); we will check this
% in the camera-ready version and ask you to change it back.

% ----- Import from AAAI ------
\usepackage{times}  % DO NOT CHANGE THIS
\usepackage{helvet} % DO NOT CHANGE THIS
\usepackage{courier}  % DO NOT CHANGE THIS
\usepackage{graphicx} % DO NOT CHANGE THIS
\usepackage{subcaption}
\usepackage{natbib}  % DO NOT CHANGE THIS AND DO NOT ADD ANY OPTIONS TO IT
\usepackage{caption} % DO NOT CHANGE THIS AND DO NOT ADD ANY OPTIONS TO IT
\frenchspacing  % DO NOT CHANGE THIS

% ----- Track 4: SIMMC -----
\usepackage{amsmath}
\usepackage{booktabs}
% \usepackage{subcaption}
\usepackage{xcolor}
\usepackage{xspace}
\usepackage{enumitem}
\usepackage{multirow, multicol}
\usepackage{flushend}

\usepackage{amsfonts}
\newcommand{\abr}[1]{\textsc{#1}}
\newcommand{\dn}{\abr{simmc }{\small 2.0}\xspace} % dataset name

\include{tex/simmc_macros}
\include{tex/space_saver}
\include{tex/shane_macros}

\usepackage[misc]{ifsym} % Letter
\newcommand*\samethanks[1][\value{footnote}]{\footnotemark[#1]}

\title{SIMMC 2.0: A Task-oriented Dialog Dataset\\for Immersive Multimodal Conversations}

\author{ \\
  \textbf{Satwik Kottur}\thanks{\hspace{5pt}Joint first authors},
  \textbf{Seungwhan Moon}\samethanks,
  \textbf{Alborz Geramifard},
  \textbf{Babak Damavandi} \\
  Facebook Reality Labs \& Facebook AI \\
  {\small \Letter}\hspace{3pt} \texttt{\{skottur,shanemoon,alborzg,babakd\}@fb.com} \\
}
\date{}



\begin{document}
\maketitle
% \begin{abstract}
% % Motivate multimodal task-oriented dialog up front
% % a. virtual assistants gain more intelligence -> will handle multimodal input
% %We envision that a new generation of
% Next generation task-oriented dialog systems need to understand conversational contexts with 
% their perceived surroundings, to effectively help users in the real-world multimodal 
% environment. 
% % b. currently we lack resources / model suites to study it.
% Existing task-oriented dialog datasets aimed towards virtual assistance fall short and do not 
% situate the dialog in the user's multimodal context.
% % c. to this end, we present a new corpus
% To overcome, we present a new dataset for Situated and Interactive Multimodal
% Conversations, \dn, which includes $11K$ task-oriented user$\leftrightarrow$assistant 
% dialogs ($117K$ utterances) in the shopping domain, grounded in immersive and photo-realistic
% scenes.


% % The dialogs are collected using a two-phase pipeline, which first generates simulated dialog 
% % flows via a novel multimodal dialog simulator we introduce, 
% % followed by manual paraphrasing of the generated utterances.
% The dialogs are collection using a two-phase pipeline:
% (1) A novel multimodal dialog simulator generates simulated dialog flows, with an emphasis on 
% diversity and richness of interactions,
% (2) Manual paraphrasing of generating utterances to draw from natural language distribution.
% % In this paper,
% \sm{
% We provide an in-depth analysis of the collected dataset, and describe in detail the four main benchmark tasks we propose for \dn.
% Our baseline model, \sk{powered by the state-of-the-art language model}, shows promising 
% results, and highlights new challenges and directions for the community to study.
% Our dataset and code will be made publicly available.}
% \end{abstract}
% %Multimodal Disambiguation, Multimodal Coreference Resolution (MM-Coref), Multimodal Dialog State Tracking (MM-DST), and Response Generation


% \section{Introduction}
% \input{sections/introduction}

% \section{Related Work}
% \label{sec:related_work}
% \input{sections/related_work}

% \section{SIMMC 2.0 Dataset}
% \label{sec:dataset}
% \input{sections/dataset}


% \subsection{SIMMC 2.0 Dataset Analysis}
% \label{sec:dataset_analysis}
% \input{sections/dataset_analysis}


% \section{Task Formulation}
% \label{sec:task_formulation}
% \input{sections/task_formulation}


% \section{Modeling \& Empirical Analysis}
% \label{sec:model_analysis}
% \input{sections/modeling}


% \textbf{Conclusions.}
% % \section{Conclusions}
% %Our \textbf{main contributions} are as follows:
% % First, 
% We present a novel dataset for the Situated and Interactive Multimodal Conversations,
% \dn{}, with $11K$ user$\leftrightarrow$assistant dialogs ($117K$ utterances) on shopping domain (fashion and furniture), grounded in situated and photo-realistic VR scenes.
% We then present a novel multimodal dialog simulator, which generates simulated dialogs grounded on diverse multimodal contexts that are automatically configured.
% Our empirical analysis with a baseline model demonstrates many new challenges that our \dn{} dataset brings, highlighting new directions of research in this area.


% \bibliography{bibliography}
% %\bibliographystyle{plainnat}
% \bibliographystyle{acl_natbib}
% \vfill
% \pagebreak
\textbf{Appendix A. Example Dialog}
\input{tex/supplementary.tex}

\end{document}
